# Supplementary material for: Part2Object: Hierarchical Unsupervised 3D Instance Segmentation
Source: arXiv:2407.10084 source file (2024-07-14)
Supplement: Supplementary file 1 [file X_suppl.tex]

\newpage
\appendix
\section*{Appendix}
In this section, we present additional implementation details, experiment results and discussions. The content structure is outlined as follows:

\begin{itemize}
% [topsep=0pt,itemsep=-1ex,partopsep=1ex,parsep=1ex]
    % \item Section~\ref{sec:prompts} - Detailed Prompts
    \item Section~\ref{sec:add_results} - Cross-dataset Generalization Results
    \item Section~\ref{sec:Implementation} - Additional Implementation Details
    \item Section~\ref{sec:case_sty} - Visualizations
    \item Section~\ref{sec:limits} - Limitations
    
\end{itemize}

\section{Cross-dataset Generalization Results}
\label{sec:add_results}
% According to the presentation in Table~\ref{supp}, we further validate the effectiveness of our method on the Scannet200 and S3DIS datasets. We train the model exclusively using the ScanNet~\cite{dai2017scannet} dataset and evaluate its class-agnostic instance segmentation performance on ScanNet200~\cite{rozenberszki2022language} and S3DIS~\cite{armeni2017joint} dataset. Compare to methods trained through full supervision, our pseudo-labels assist the model in learning more generalizable 3D object knowledge, resulting in improvements of 1.6\% and 2.9\% in the head and common categories. And our method also achieves competitive results with the fully supervised approach in the tail categories. The results on the S3DIS~\cite{armeni2017joint} dataset also demonstrate that our method can achieve performance comparable to or even surpassing fully supervised methods on a more extensive dataset.

\textbf{Datasets.} ScanNet200~\cite{rozenberszki2022language} extends ScanNet~\cite{dai2017scannet} by adding annotations for a larger number of categories which are split into common and tail categories based on the imbalance in category distribution. S3DIS~\cite{armeni2017joint} is a large-scale indoor point cloud dataset, consisting of six different areas in three distinct campus buildings, totaling 272 scenes. Each scene is annotated with semantic and instance segmentation labels for 13 categories.

In accordance with the presentation in Table~\ref{supp}, we further validate the effectiveness of our method in terms of cross-dataset generalization on the ScanNet200~\cite{rozenberszki2022language} and S3DIS~\cite{armeni2017joint} datasets. We choose ScanNet~\cite{dai2017scannet} as the source domain and ScanNet200~\cite{rozenberszki2022language} as well as S3DIS~\cite{armeni2017joint} as the target domains, testing the class-agnostic instance segmentation performance. Compared to methods trained through full supervision, our pseudo-labels assist the model in learning more generalizable 3D object knowledge, resulting in improvements of 1.6\% and 2.9\% in the head and common categories, respectively. Moreover, our method achieves competitive results with the fully supervised approach in the tail category. The results on the S3DIS~\cite{armeni2017joint} dataset also demonstrate that our method can achieve performance comparable to or even surpassing fully supervised methods on a more extensive dataset.

\begin{table}[htbp]
    \centering
    % \tin
    
    % \tabcolsep=0.5cm
    % \setlength{\tabcolsep}{3mm}{
    \resizebox{0.5\textwidth}{!}{
    \begin{tabular}{l|ccc}
        \Xhline{2pt}
        \multirow{2}{*}{ScanNet~\cite{dai2017scannet} $\rightarrow$ ScanNet200~\cite{rozenberszki2022language}} & Head & Common & Tail \\
&  \textcolor{gray}{\textbf{AP@50}} & \textcolor{gray}{\textbf{AP@50}} & \textcolor{gray}{\textbf{AP@50}} \\
        
        % Scannet200 & AP & AP@50 & AP@25 \\ 
        \hline
        
        Mask3D~\cite{Schult23mask3d} (fully supervised) & 29.4 & 26.3 & \textbf{25.6} \\
        \textbf{Ours} (unsupervised) & \textbf{31.0} & \textbf{29.2} & 23.1 \\
        \Xhline{1.5pt}
        ScanNet~\cite{dai2017scannet} $\rightarrow$ S3DIS~\cite{armeni2017joint}  & AP & AP@50 & AP@25 \\ 
        \hline
        Mask3D~\cite{Schult23mask3d} (fully supervised) &\textbf{13.1} & 19.2 &  26.0 \\
        \textbf{Ours}(unsupervised) & 11.5 & \textbf{23.9} & \textbf{39.2} \\
        % \Xhline{1.5pt}
        % dataset & AP & AP@50 & AP@25 \\ 
        % \hline
        % supervised model 1& 30 & 30 & 30 \\ 
        % supervised model 2& 30 & 30 & 30 \\
        % supervised model 3& 30 & 30 & 30 \\
        % \textbf{Ours} & \textbf{20} & \textbf{20} & \textbf{20} \\
        \Xhline{2pt}
    \end{tabular} 
    }
    \caption{Cross-dataset Generalization Results on S3DIS~\cite{armeni2017joint} and ScanNet200~\cite{rozenberszki2022language}.}
    \label{supp}
    % }
    % }
\end{table}

\section{Additional Implementation Details}
\label{sec:Implementation}
Regarding specific hierarchical clustering algorithm, we demonstrate one layer of the clustering method through Algorithm~\ref{algorithm1}.
\begin{algorithm}[htbp]
    \SetAlgoLined
    \KwData{clusters $\{\mathbf{P}^{l}_{i}\}_{i=1}^{n^{l}}$, cluster features $\{f_{i}^{l}\}_{i=1}^{n^{l}}$, discovered 3D objects $\{b_{i}\}_{i=1}^{H}$, point features $\{f_{i,j}\}_{j=1}^{n_{i}^{l}}$}
    \KwResult{clusters $\{\mathbf{P}^{l+1}_{i}\}_{i=1}^{n^{l+1}}$, cluster features $\{f_{i}^{l+1}\}_{i=1}^{n^{l+1}}$}

    % // applying 2D priors \\
    \For{ every cluster $\mathbf{P}^{l}_{i}$ \Kwdo}
    {
        find objects $b_{j}$, that $\mathbf{P}^{l}_{i}$ in $b_{i}$ \\
        label $l_{i}$ \leftarrow $j$ \\
    }

    % $sim\_matrix \leftarrow sim(\{\Vec{h}_{i}\}_{i=0}^{S_{l}}, \{\Vec{h}_{i}\}_{i=0}^{S_{l}})$
    
    % $sim\_matrix[\sim I_{S_{l}}] \leftarrow 0$ \\
    % $pairs \leftarrow argsort(sim\_matrix)$ \\
    % // perform clustering \\
    \For{every pairs $(i, j)$ \Kwdo}{
        % \If{$sim(f_{i}^{l}, f_{j}^{l})$ not in topK pairs}{Continue}
        % \If{$I_{l}(i, j)$ != Ture}{Continue}
        \If{$sim(f_{i}^{l}, f_{j}^{l})$ in \textnormal{topK} and $adj(\mathbf{P}^{l}_{i}, \mathbf{P}^{l}_{j})$ and $l_{i} == l_{j}$ }{
        $\mathbf{P}^{l+1}_{i} \leftarrow \mathbf{P}^{l}_{i} \cup \mathbf{P}^{l}_{j}$\\
        % \If{$l_{j} != None$}{$l_{i} \leftarrow l_{j}$}\\
        % $I_{l+1}[i] \leftarrow I_{l}[i] \cup I_{l}[j]$ \\
        }
        % \eIf{$l_{i} != l_{j} \land l_{i} != None \land l_{j} != None$}{
        %     Continue
        % }{
        % $\mathbf{P}^{l+1}_{i} \leftarrow \mathbf{P}^{l}_{i} \cup \mathbf{P}^{l}_{j}$\\
        % % \If{$l_{j} != None$}{$l_{i} \leftarrow l_{j}$}\\
        % $I_{l+1}[i] \leftarrow I_{l}[i] \cup I_{l}[j]$ \\
        % Delete $I_{l}[j]$
        % }
    }

    % Obtain $S_{l+1}$ regions $\{\mathbf{P}^{\prime}_{i}\}_{i=1}^{S_{l+1}}$ and adj\_matrix $I_{S_{l+1}}$\\
    
    % // update cluster features \\
    \For{every new cluster $\mathbf{P}^{l+1}_{i}$}{
    % $ \Bar{f_{i}^{l+1}} \leftarrow  avgpool(\{f_{i,j}^{l}\}_{j=1}^{n_{i}^{l}})$ \\
    % $w \leftarrow sim(\Bar{f_{i}^{l+1}}, \{f_{i,j}^{l}\}_{j=1}^{n_{i}^{l}})$ \\
    % $ f_{i}^{l+1} \leftarrow weighted\_avg(\{f_{i,j}^{l}\}_{j=1}^{n_{i}^{l}}, w)$
    $f_{i}^{l+1} \leftarrow update\_cluster\_features(\{f_{i,j}\}_{j=1}^{n_{i}^{l+1}})$
    }
    
    % Obtain $S_{l+1}$ region features $\{\Vec{h}_{i}\}_{i=0}^{S_{l+1}}$ \\
    \textbf{return} $\{\mathbf{P}^{l+1}_{i}\}_{i=1}^{n^{l+1}}$, $I_{l+1} \in \mathbb{R}^{n^{l+1} \times n^{l+1}}$, $\{f_{i}^{l+1}\}_{i=1}^{n^{l+1}}$

    \caption{Hierarchical Clustering in Layer l}
    \label{algorithm1}
\end{algorithm}

Here, $sim$ represents the cosine similarity between two features, and $adj$ indicates whether two clusters are adjacent. In this context, we define the distance between two clusters as the distance between their nearest points, and clusters with distances less than $\tau$, which is 0.05, are considered adjacent clusters. Additionally, similar to the description in Section 3.2, we update the cluster features by recalculating the features of the newly clustered points.

% Algorithm~\ref{algorithm1} shows the detailed procedure to produce $S_{i+1}$ regions from $S_{i}$ regions in grouping layer $i$.  Specifically, given a set of $S_{i}$ regions and their adjacency matrix $I_{i}$, we first assigned a distinct label to the regions covered by the bounding boxes acting as object priors. Subsequently, based on the feature similarity between adjacent regions, we selected the top K pairs of neighboring regions as clustering candidates. For each pair of neighboring regions in clustering candidates, if the regions belonged to different labels, indicating they were part of different instances, they were removed from the clustering candidates. Finally, the remaining pairs of neighboring regions in the clustering candidates were merged one by one, and then the region features and adjacency matrix were updated, resulting in $S_{i+1}$ regions after clustering.

\section{Visualizations}
\label{sec:case_sty}

\noindent\textbf{Part Results} Figure~\ref{fig:part} demonstrates that our part2obj model can decompose different objects into corresponding part results. Thanks to the object-level decoder, part-level decoder, and our ``targeting the objective and advancing" pseudo-label generation strategy, we can obtain reasonable part masks.
Although we can obtain reasonable parts for most objects, constrained by the limitations of unsupervised learning, we may fail in some certain objects, such as the chair in the line 4 of the figure. Improving the precise detection of different components within objects and obtaining more accurate part masks is a direction for future refinement.

\noindent\textbf{Qualitative Comparisons With Other Methods} In Figure~\ref{fig:vis}, we conduct qualitative comparisons on ScanNet~\cite{dai2017scannet}. Compared to the Felzenswalb~\cite{felzenszwalb2004efficient} method and the 2D method CutLER's~\cite{wang2023cut} projection masks, our results can simultaneously handle objects of different sizes and structural complexities, avoiding under-segmentation and over-segmentation. This approach achieves complete and clear object masks.
Specifically, for structurally simple objects, such as a table (line 1), our masks are more accurate at the edges. For structurally complex objects, like a bookshelf (line 6), our method not only identifies this as an object but also obtains accurate masks. Additionally, we can detect smaller objects, such as a backpack (line 3), and avoid splitting larger objects, like a sofa, into many parts.

\noindent\textbf{Qualitative Comparisons With Different Clustering Methods} In Figure~\ref{fig:cluster}, we present the results of single-layer clustering under different hyperparameters, clustering results without object priors, and our clustering results. Observations reveal that, under specific hyperparameters, single-layer clustering tends to handle only one size of object. The hierarchical clustering without object priors still struggles to identify the majority of objects. However, our clustering algorithm effectively handles most objects.

% \twocolumn[\begin{figure}[t]
% \centering
% \includegraphics[width=0.45\textwidth]{figs/vis.pdf}
% \caption{}
% \vspace{-3mm}
% \label{fig:vis}
% \end{figure}]

\begin{figure}[htbp]
\centering
% \includesvg[width=0.8\textwidth]{figs/appex1.png}
\includegraphics[width=0.5\textwidth]{figs/part_vi.png}

\caption{Different objects and their corresponding part results.}
\vspace{-3mm}
\label{fig:part}
\end{figure}

\begin{figure*}[htbp]
\centering
% \includesvg[width=0.8\textwidth]{figs/appex1.png}
\includegraphics[width=0.98\textwidth]{figs/appex1.png}

\caption{Qualitative comparisons on ScanNet~\cite{dai2017scannet}. Compared to the Felzenswalb~\cite{felzenszwalb2004efficient} method and the 2D method CutLER's~\cite{wang2023cut} projection masks.}
\vspace{7mm}
\label{fig:vis}
\end{figure*}

\begin{figure*}[htbp]
\centering
% \includesvg[width=0.8\textwidth]{figs/appex1.png}
\includegraphics[width=0.98\textwidth]{figs/cluster2.png}

\caption{The comparison of clustering results between different clustering methods.}
\vspace{-3mm}
\label{fig:cluster}
\end{figure*}

\section{Limitations}
\label{sec:limits}

The 2D features in this study is derived from self-supervised models DINO~\cite{caron2021emerging_dino} and CutLER~\cite{wang2023cut}. Due to potential biases and controversies in the training data of these models, our model may be influenced by these issues. This could result in limitations to the performance of the model, particularly in applications involving ethics and fairness.

Despite achieving superior performance in multiple experimental settings, the generalization capability of the model needs more comprehensive validation across a wider range of tasks and domains. Further research and validation are required to investigate whether the model is equally effective in other domains and applicable to more complex scenarios.

Given these limitations, future research efforts could focus on enhancing the model's robustness and improving its performance in diverse data domains and ethical considerations.
