# Supplementary material for: Part2Object: Hierarchical Unsupervised 3D Instance Segmentation
Source: arXiv:2407.10084 source file (2024-07-14)
Supplement: Supplementary file 2 [file appendix_p_code.tex]

% \lstset{style=colab}
% \begin{lstlisting}[language=ColabPython]
% # topk_pair is a list: each element represents a pair of cluster IDs that satisfy Equ 3.
% # obj_ids is a list: it orders to store cluster id that is a object.
% # objectness_prior_bboxes is a list: each element represents an axis-aligned bounding box (AABB) acquired by Section 3.2.
% # coords is an np.ndarray: it stores the (x, y, z) coordinates of each point, and its shape is [Num_Points, 3].
% # point2cluster is an np.ndarray: it stores the cluster ID to which each point belongs, and its shape is [number of points, 1].
% # iou_threshold is a float: if the Intersection over Union (IOU) between a cluster bbox and any bbox in objectness_prior_bboxes is greater than iou_threshold, consider this cluster as an object.
% topk_pair = [...]
% obj_ids = []
% objectness_prior_bboxes = [...]
% coords = ...
% point2cluster = ...
% iou_threshold = 0.6

% for i,j in topk_pair:
%     if i != j and i not in obj_id:
%         # merge cluster
%         point2cluster[point2cluster == j] = i
%         # judge whether it is an object
%         cluster_coords = coords[point2cluster == i]
%         cluster_bbox = np.concatenate((np.min(cluster_coords, axis=0), np.max(cluster_coords, axis=0)), axis=0).reshape(1, 6)
%         ious = batch_box_iou(marged_bbox, boxes)
%         if ious.max() > iou_threshold:
%             obj_ids.append(i)
% \end{lstlisting}

\begin{algorithm}[htbp]
    \SetAlgoLined
    \KwData{clusters $\{c^{t}_{i}\}_{i=1}^{N_{t}}$, cluster features $\{\boldsymbol{f}_{i}^{t}\}_{i=1}^{N_{t}}$, \\
    3D objectness priors $B^{3D}$
    }
    \KwResult{clusters $\{c^{t+1}_{k}\}_{k=1}^{N_{t+1}}$, cluster features $\{\boldsymbol{f}_{k}^{t+1}\}_{k=1}^{N_{t+1}}$}

    iou\_threshold $\leftarrow$ $0.6$ \\

    \For{every pairs $(i, j)$ }{
        \If{$ \text{rank}(\text{sim}(\boldsymbol{f}_{i}^{t}, \boldsymbol{f}_{j}^{t})) \leq K $ \textbf{and} $dist({c}^{t}_{i}, {c}^{t}_{j}) \leq T$}{
            \If{not $stopCriteria({c}^{t}_{i},{c}^{t}_{j},B^{3D})$ }{
                ${c}^{t+1}_{k} \leftarrow {c}^{t}_{i}\cup {c}^{t}_{j}$
            }
        }
    }
    \For{every new cluster ${c}^{t+1}_{k}$}{
        $\boldsymbol{f}_{k}^{t+1} \leftarrow $\texttt{FU}$({c}^{t+1}_{k})$
    }
    \textbf{return} $\{{c}^{t+1}_{k}\}_{i=1}^{N_{t+1}}$,
    $\{\boldsymbol{f}_{i}^{t+1}\}_{i=1}^{N_{t+1}}$
    \caption{\textcolor{black}{Hierarchical Clustering in Layer $t$}}
    \label{algorithm1}
\end{algorithm}
\noindent
Here $stopCriteria$ denotes the algorithm from line 263 in submitted paper.

    % \For{ every cluster ${c}^{l}_{i}$ }
    % {
    %     \If{max(batch\_box\_iou(${c}^{l}_{i}$, $B^{3D}$)) $\geq$ iou\_threshold}{
    %         $l_{i}$ $\leftarrow$ $1$
    %     }
    % }
