# Supplementary material for: Part2Object: Hierarchical Unsupervised 3D Instance Segmentation
Source: arXiv:2407.10084 source file (2024-07-14)
Supplement: Supplementary file 3 [file appendix_table1.tex]

\begin{table}[h]
\centering
\caption{\textbf{The hyper-parameter configuration for training Hi-Mask3D}, where * denote data-efficient setting.}
\begin{tabular}{c|ccc}
\hline
\textbf{Configuration} & \textbf{ScanNet} & \textbf{ScanNet*} & \textbf{S3DIS*} \\
\hline
Optimizer & AdamW & AdamW & AdamW \\
Learning rate (LR) & $1\times10^{-4}$ & $1\times10^{-4}$  & $1\times10^{-4}$\\
Scheduler & OneCycleLR & OneCycleLR & OneCycleLR \\
Batch size & 4 & 4 & 4 \\
Epochs & 600 & 600 & 600 \\
Part Queries Number & $300$ & $300$ & $300$ \\
Object Queries Number & $150$ & $150$ & $150$ \\
Voxel Size & $0.02$ & $0.02$ & $0.02$ \\
%With Segment & Yes & Yes & No \\
Filter Out Classes & None & Wall, Floor & None \\

\hline
\end{tabular}
\label{app_tab1}
% \vspace{-5mm}
\end{table}
