# Supplementary material for: Part2Object: Hierarchical Unsupervised 3D Instance Segmentation
Source: arXiv:2407.10084 source file (2024-07-14)
Supplement: Supplementary file 5 [file appendix_table2_s3dis.tex]

\begin{tabular}{l|cc|cc|cc}\toprule
S3DIS 6 fold ~\cite{s3dis} 
& \multicolumn{2}{c}{Area 1} & \multicolumn{2}{c}{Area 2} & \multicolumn{2}{c}{Area 3}  \\
\cmidrule(lr){2-3} \cmidrule(lr){4-5} \cmidrule(lr){6-7}
Methods & m@25 & m@50 
        & m@25 & m@50 
        & m@25 & m@50 \\
\midrule
 Mask3D~\cite{Schult23mask3d} 
 & $19.0$ & $12.4$ 
 & $15.8$ & $10.6$ 
 & $19.9$ & $13.1$ \\
 
\rowcolor{gray}  Ours 
 & $25.7$ & $17.1$ 
 & $24.5$ & $16.4$ 
 & $24.0$ & $16.4$ \\
\bottomrule
\end{tabular}

\begin{tabular}{l|cc|cc|cc}\toprule
S3DIS 6 fold ~\cite{s3dis} 
&  \multicolumn{2}{c}{Area 4} & \multicolumn{2}{c}{Area 5} & \multicolumn{2}{c}{Area 6} \\
\cmidrule(lr){2-3} \cmidrule(lr){4-5} \cmidrule(lr){6-7}
Methods & m@25 & m@50
        & m@25 & m@50
        & m@25 & m@50\\
\midrule
 Mask3D~\cite{Schult23mask3d} 
 & $16.4$ & $10.9$ 
 & $16.8$ & $11.5$ 
 & $17.6$ & $11.6$ \\
 
\rowcolor{gray}  Ours 
 & $24.8$ & $17.0$ 
 & $21.5$ & $14.4$ 
 & $26.7$ & $17.6$ \\
\bottomrule
\end{tabular}
\vspace{-0.3cm}
