# Supplementary material for: Part2Object: Hierarchical Unsupervised 3D Instance Segmentation
Source: arXiv:2407.10084 source file (2024-07-14)
Supplement: Supplementary file 6 [file appendix_table2_scannet200.tex]

\begin{tabular}{l|ccc|ccc|ccc}\toprule
ScanNet200 val~\cite{scannet200} &\multicolumn{3}{c}{Head} &\multicolumn{3}{c}{Common} &\multicolumn{3}{c}{Tail} \\
\cmidrule(lr){2-4} \cmidrule(lr){5-7} \cmidrule(lr){8-10}
Methods &  m@25 & m@50 &mAP &  m@25 & m@50 &mAP &  m@25 & m@50 &mAP\\
\midrule
 Mask3D~\cite{Schult23mask3d} 
 & $36.4$ & $25.8$ & $15.7$
 & $26.0$ &$19.5$ &$11.2$
 & $23.6$ &$18.7$ &$10.7$\\
 
\rowcolor{gray}  Ours 
& $64.8$ & $35.8$ & $16.8$ 
& $53.8$ & $30.5$ & $12.0$ 
& $45.2$ & $24.5$ & $9.8$ \\
\bottomrule
\end{tabular}
