# Supplementary material for: Part2Object: Hierarchical Unsupervised 3D Instance Segmentation
Source: arXiv:2407.10084 source file (2024-07-14)
Supplement: Supplementary file 7 [file appendix_table3_1.tex]

\newcommand{\fig}[2][1]{\includegraphics[width=#1\linewidth]{#2}}

\begin{tabular}{cc}

\rotatebox{90}{\phantom{10000} Input} & \fig[.99]{eccv/figs/appendix_fig/vis/r1_1.png} \\
\rotatebox{90}{\phantom{0} Felzenswalb~\cite{felzenszwalb2004efficient}} &\fig[.99]{eccv/figs/appendix_fig/vis/r1_2.png}\\
\rotatebox{90}{\phantom{0} CutLER~\cite{wang2023cut}} &\fig[.99]{eccv/figs/appendix_fig/vis/r1_3.png} \\
\rotatebox{90}{\phantom{0} Pseudo Label} &\fig[.99]{eccv/figs/appendix_fig/vis/r1_4.png} \\
\rotatebox{90}{\phantom{12000} Ours} &\fig[.99]{eccv/figs/appendix_fig/vis/r1_5.png} \\
\rotatebox{90}{\phantom{34000} GT} &\fig[.99]{eccv/figs/appendix_fig/vis/r1_6.png} \\

\end{tabular}
