# Supplementary material for: Part2Object: Hierarchical Unsupervised 3D Instance Segmentation
Source: arXiv:2407.10084 source file (2024-07-14)
Supplement: Supplementary file 8 [file appendix_table3_2.tex]

\newcommand{\fig}[2][1]{\includegraphics[width=#1\linewidth]{#2}}

\begin{tabular}{cc}

\rotatebox{90}{\phantom{14000} Input} & \fig[.99]{eccv/figs/appendix_fig/vis/r2_1.png} \\
\rotatebox{90}{ \phantom{10}Felzenswalb~\cite{felzenszwalb2004efficient}} &\fig[.99]{eccv/figs/appendix_fig/vis/r2_2.png}\\
\rotatebox{90}{ \phantom{10}CutLER~\cite{wang2023cut}} &\fig[.99]{eccv/figs/appendix_fig/vis/r2_3.png} \\
\rotatebox{90}{ \phantom{10}Pseudo Label} &\fig[.99]{eccv/figs/appendix_fig/vis/r2_4.png} \\
\rotatebox{90}{ \phantom{12000}Ours} &\fig[.99]{eccv/figs/appendix_fig/vis/r2_5.png} \\
\rotatebox{90}{\phantom{20000} GT} &\fig[.99]{eccv/figs/appendix_fig/vis/r2_6.png} \\

\end{tabular}
