# Supplementary material for: Part2Object: Hierarchical Unsupervised 3D Instance Segmentation
Source: arXiv:2407.10084 source file (2024-07-14)
Supplement: Supplementary file 9 [file appendix_table4.tex]

\newcommand{\fig}[2][1]{\includegraphics[width=#1\linewidth]{#2}}

\begin{tabular}{cc}

\rotatebox{90}{\phantom{26000} Input} & \fig[.99]{figs/appendix_fig/vis_part/l1.png} \\
\rotatebox{90}{\phantom{26000}$\hat{P}^{\text{Part}}$} &\fig[.99]{figs/appendix_fig/vis_part/l2.png}\\
\rotatebox{90}{ \phantom{16000}$P^{\text{Part}}$} &\fig[.99]{figs/appendix_fig/vis_part/l3.png} \\
\rotatebox{90}{ \phantom{16000}$\hat{P}^{\text{Object}}$} &\fig[.99]{figs/appendix_fig/vis_part/l4.png} \\
\rotatebox{90}{ \phantom{16000}$P^{\text{Object}}$} &\fig[.99]{figs/appendix_fig/vis_part/l5.png} \\
\rotatebox{90}{ \phantom{90000}GT} &\fig[.99]{figs/appendix_fig/vis_part/l6.png} \\

\end{tabular}
